# Supplementary material for: The energy-spectrum of bicompatible sequences
Source: arXiv:1910.00190 source file (2019-10-01)
Supplement: Supplementary file 1 [file SupplementaryMaterial1.pdf]

# THE ENERGY-SPECTRUM OF BICOMPATIBLE SEQUENCES: SUPPLEMENTARY MATERIAL

## 1. Proofs

**Lemma 1.** *Let $X$ be an irreducible substructure of a bistructure without overlaps and crossing arcs. contains a unique maximal arc with respect to $\prec_B$.*

*Proof.* Suppose that is not the case. Then, without loss of generality we can assume $X$ contains exactly two maximal arcs, denoted by $m_1$ and $m_2$. We define two sets of loops $X_1 = \{L_{p_i} \mid p_i \prec_B m_1\}$ and $X_2 = \{L_{p_i} \mid p_i \prec_B m_2\}$. By definition $X_1 \cup X_2$ is a bi-partition of $X$. However, any loop in $X_1$ will have trivial intersection with any loop in $X_2$, since there are no crossing arcs in $X$. This contradicts the fact that $X$ is irreducible. Thus $X$ has a unique maximal arc.

□

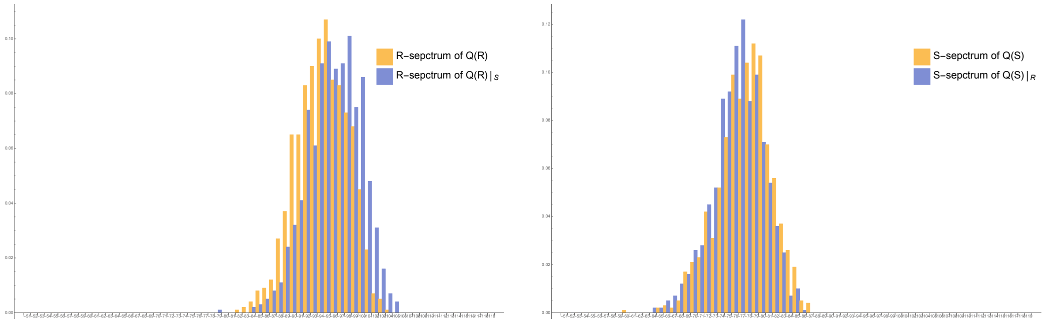


R-spectrum of `xpt` S-spectrum of `xpt`

Figure 1. The $R$- and $S$ spectra of the riboswitch structure pair, `xpt`. upper left: $f^R_{Q(R)}$ versus $f^R_{Q(R)|_S}$ for `xpt`. upper right: $f^S_{Q(S)}$ versus $f^S_{Q(S)|_R}$ for `xpt`.

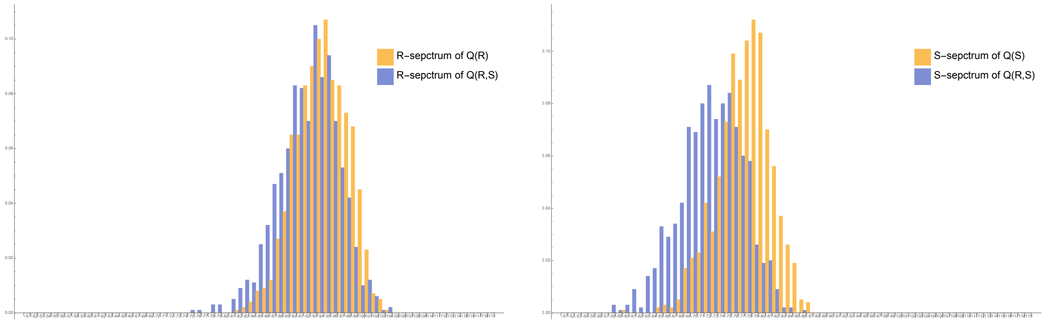


R-spectrum of `xpt` S-spectrum of `xpt`

Figure 2. The $R$- and $S$ spectra of the riboswitch structure pair, `xpt`. (LHS): $f^R_{Q(R)}$ versus $f^R_{Q(R,S)}$ for `xpt`. (RHS): $f^S_{Q(S)}$ versus $f^S_{Q(R,S)}$ for `xpt`.

## 2. $R$- and $S$-spectra for additional riboswitches

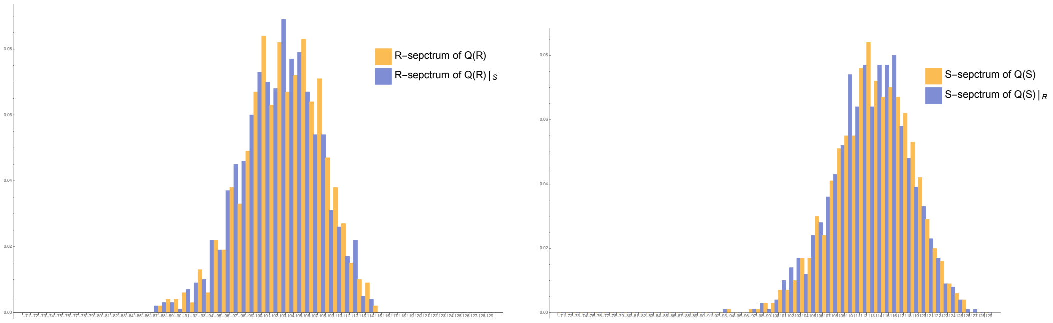


R-spectrum of mgt S-spectrum of mgt

FIGURE 3. The $R$- and $S$ spectra of the riboswitch structure pair, mgt. upper left: $f^R_{Q(R)}$ versus $f^R_{Q(R)|_S}$ for mgt. upper right: $f^S_{Q(S)}$ versus $f^S_{Q(S)|_R}$ for mgt.

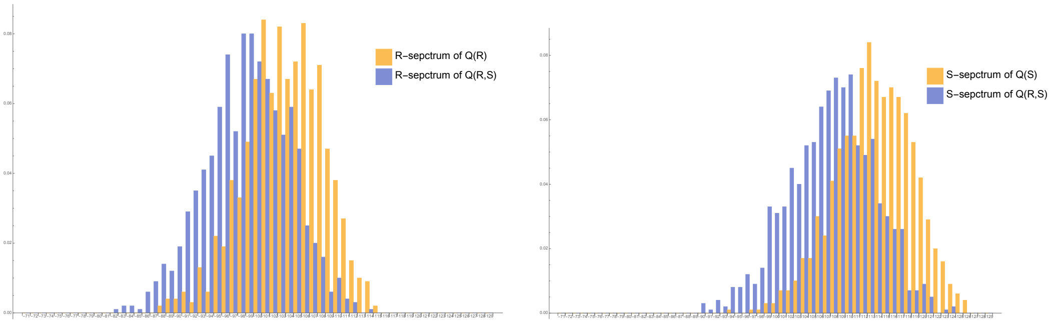


R-spectrum of mgt S-spectrum of mgt

FIGURE 4. The $R$- and $S$ spectra of the riboswitch structure pair, mgt. (LHS): $f^R_{Q(R)}$ versus $f^R_{Q(R,S)}$ for mgt. (RHS): $f^S_{Q(S)}$ versus $f^S_{Q(R,S)}$ for mgt.

## 3. $R$- AND $S$-SPECTRA FOR ADDITIONAL RANDOM STRUCTURE PAIRS

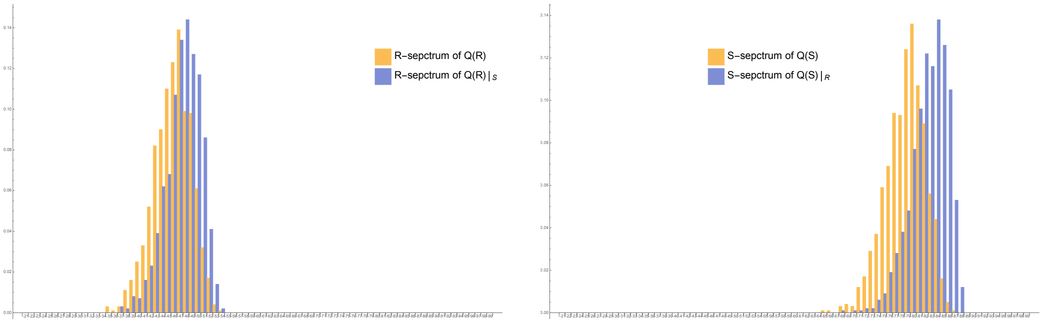


R-spectrum of `VEGFA` S-spectrum of `VEGFA`

FIGURE 5. The $R$- and $S$ spectra of the riboswitch structure pair, `VEGFA`. upper left: $f^R_{Q(R)}$ versus $f^R_{Q(R)|_S}$ for `VEGFA`. upper right: $f^S_{Q(S)}$ versus $f^S_{Q(S)|_R}$ for `VEGFA`.

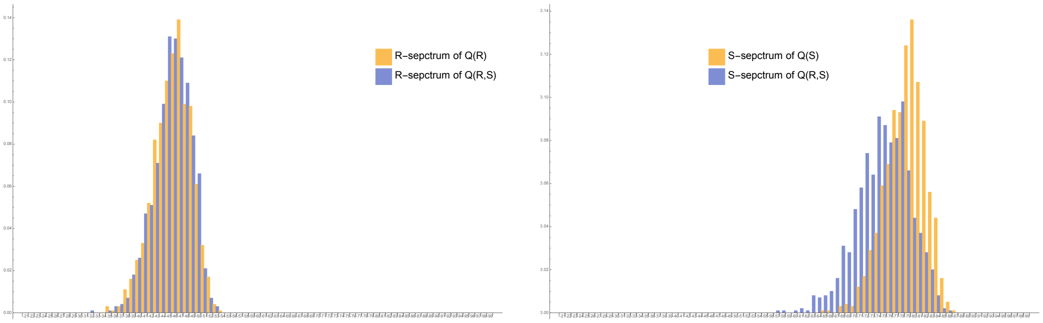


R-spectrum of `VEGFA` S-spectrum of `VEGFA`

FIGURE 6. The $R$- and $S$ spectra of the riboswitch structure pair, `VEGFA`. (LHS): $f^R_{Q(R)}$ versus $f^R_{Q(R,S)}$ for `VEGFA`. (RHS): $f^S_{Q(S)}$ versus $f^S_{Q(R,S)}$ for `VEGFA`.

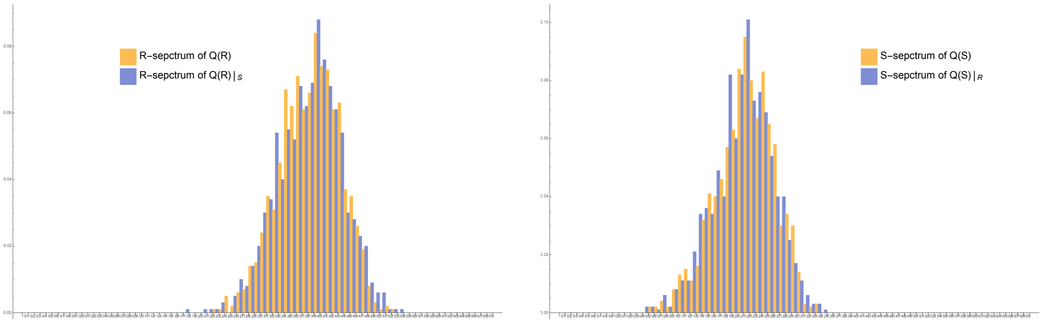


R-spectrum of `lys` S-spectrum of `lys`

FIGURE 7. The $R$- and $S$ spectra of the riboswitch structure pair, `lys`. upper left: $f^R_{Q(R)}$ versus $f^R_{Q(R)|_S}$ for `lys`. upper right: $f^S_{Q(S)}$ versus $f^S_{Q(S)|_R}$ for `lys`.

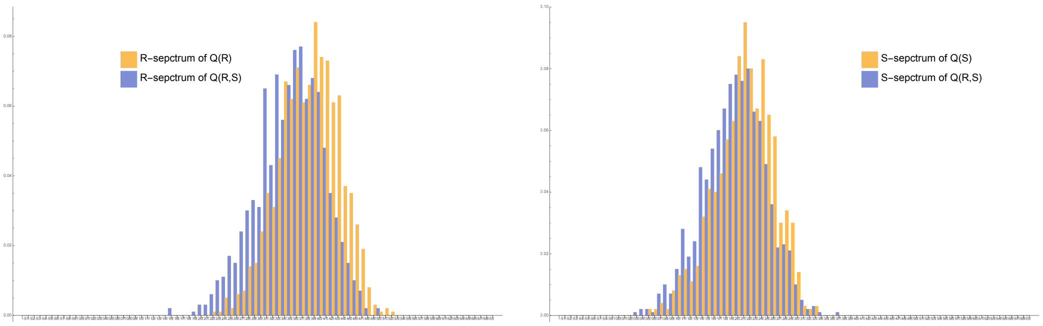


R-spectrum of `lys` S-spectrum of `lys`

FIGURE 8. The $R$- and $S$ spectra of the riboswitch structure pair, `lys`. (LHS): $f^R_{Q(R)}$ versus $f^R_{Q(R,S)}$ for `lys`. (RHS): $f^S_{Q(S)}$ versus $f^S_{Q(R,S)}$ for `lys`.

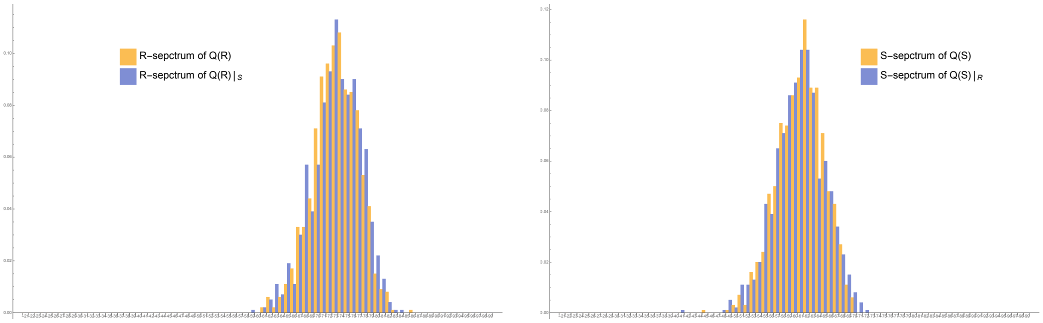


R-spectrum of `sam` S-spectrum of `sam`

FIGURE 9. The $R$- and $S$ spectra of the riboswitch structure pair, `sam`. upper left: $f^R_{Q(R)}$ versus $f^R_{Q(R)|_S}$ for `sam`. upper right: $f^S_{Q(S)}$ versus $f^S_{Q(S)|_R}$ for `sam`.

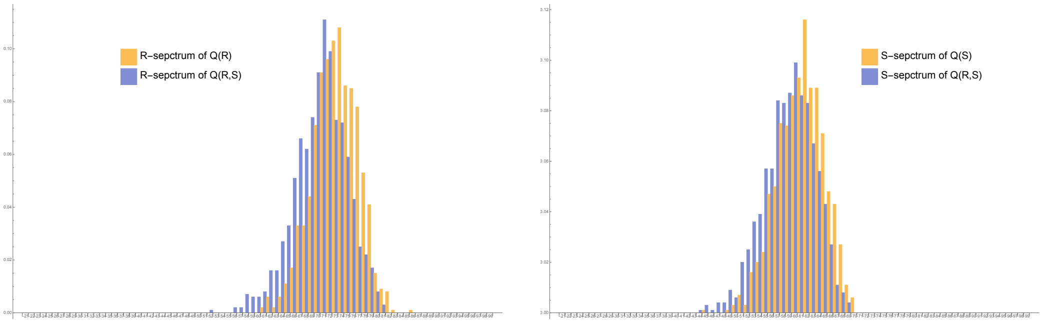


R-spectrum of `sam` S-spectrum of `sam`

FIGURE 10. The $R$- and $S$ spectra of the riboswitch structure pair, `sam`. (LHS): $f^R_{Q(R)}$ versus $f^R_{Q(R,S)}$ for `sam`. (RHS): $f^S_{Q(S)}$ versus $f^S_{Q(R,S)}$ for `sam`.

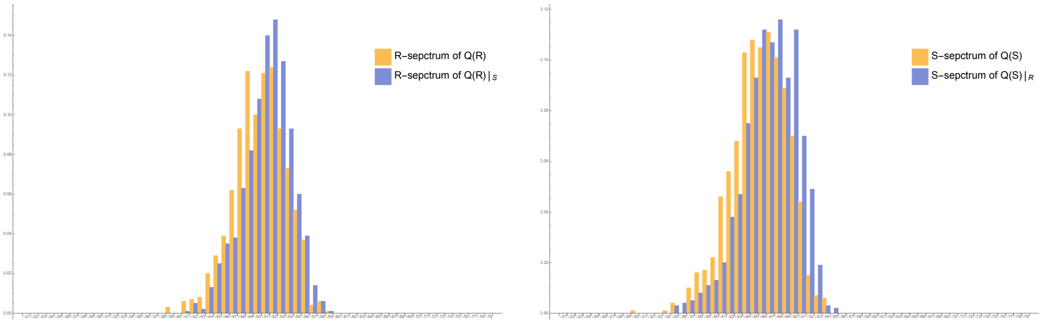


R-spectrum of `rand12` S-spectrum of `rand12`

FIGURE 11. The $R$- and $S$ spectra of the riboswitch structure pair, `rand12`. upper left: $f^R_{Q(R)}$ versus $f^R_{Q(R)|_S}$ for `rand12`. upper right: $f^S_{Q(S)}$ versus $f^S_{Q(S)|_R}$ for `rand12`.

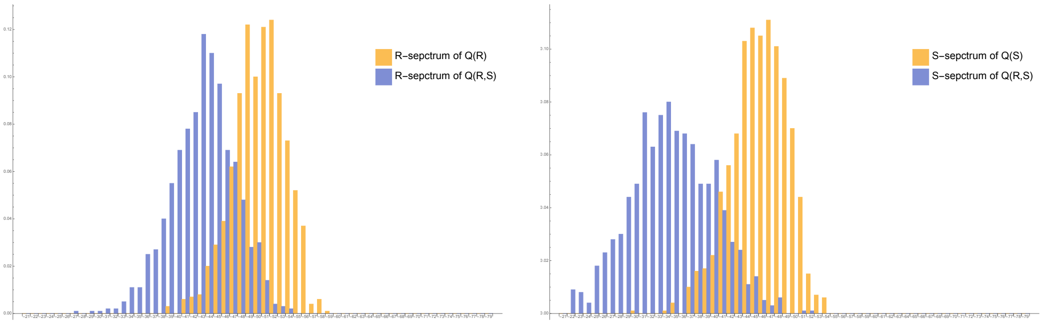


R-spectrum of `rand12` S-spectrum of `rand12`

FIGURE 12. The $R$- and $S$ spectra of the riboswitch structure pair, `rand12`. (LHS): $f^R_{Q(R)}$ versus $f^R_{Q(R,S)}$ for `rand12`. (RHS): $f^S_{Q(S)}$ versus $f^S_{Q(R,S)}$ for `rand12`.

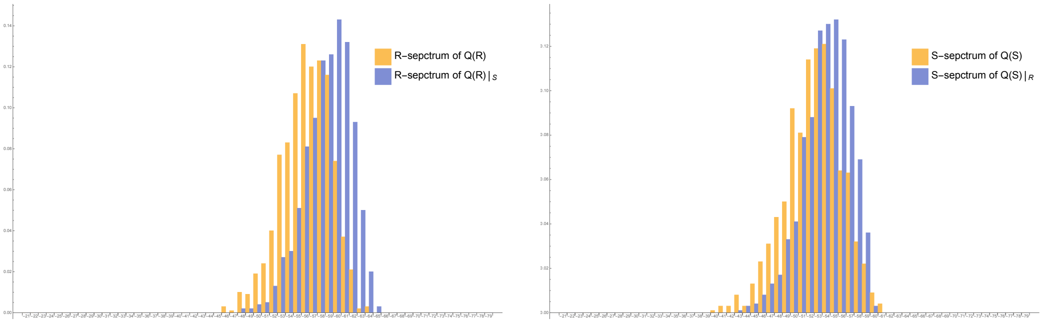


R-spectrum of `rand13` S-spectrum of `rand13`

FIGURE 13. The $R$- and $S$ spectra of the riboswitch structure pair, `rand13`. upper left: $f^R_{Q(R)}$ versus $f^R_{Q(R)|_S}$ for `rand13`. upper right: $f^S_{Q(S)}$ versus $f^S_{Q(S)|_R}$ for `rand13`.

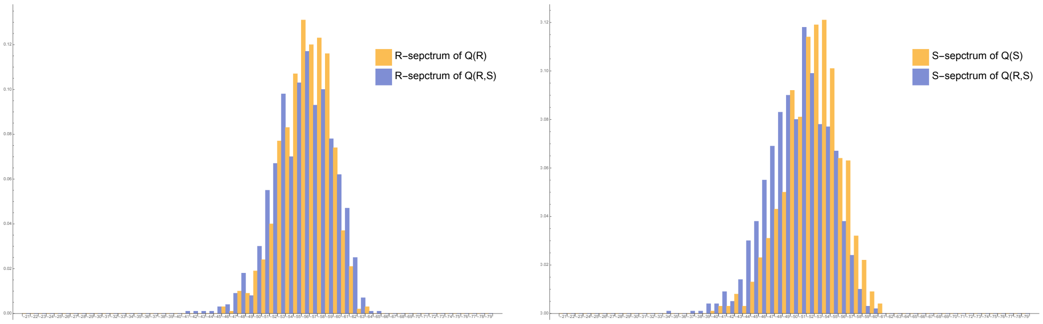


R-spectrum of `rand13` S-spectrum of `rand13`

FIGURE 14. The $R$- and $S$ spectra of the riboswitch structure pair, `rand13`. (LHS): $f^R_{Q(R)}$ versus $f^R_{Q(R,S)}$ for `rand13`. (RHS): $f^S_{Q(S)}$ versus $f^S_{Q(R,S)}$ for `rand13`.

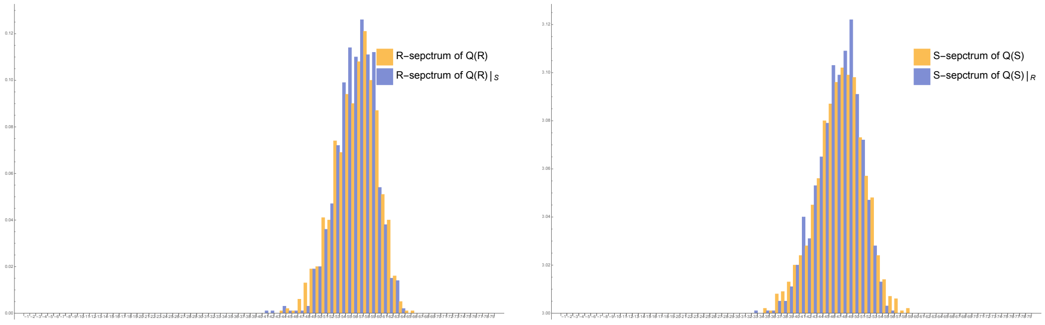


R-spectrum of `rand14` S-spectrum of `rand14`

FIGURE 15. The $R$- and $S$ spectra of the riboswitch structure pair, `rand14`. upper left: $f^R_{Q(R)}$ versus $f^R_{Q(R)|_S}$ for `rand14`. upper right: $f^S_{Q(S)}$ versus $f^S_{Q(S)|_R}$ for `rand14`.

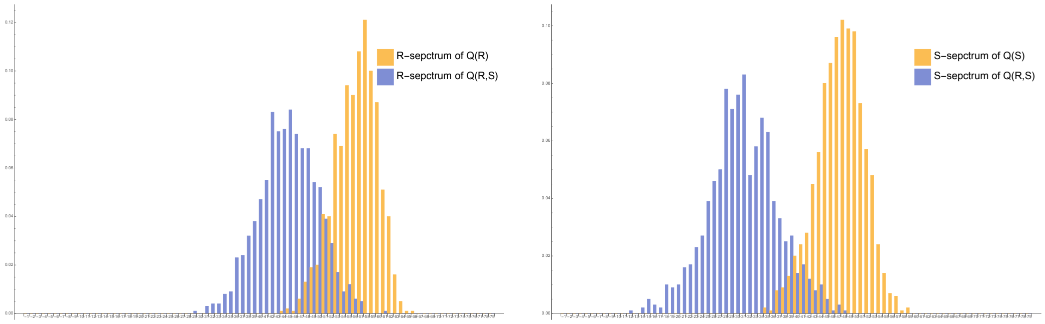


R-spectrum of `rand14` S-spectrum of `rand14`

FIGURE 16. The $R$- and $S$ spectra of the riboswitch structure pair, `rand14`. (LHS): $f^R_{Q(R)}$ versus $f^R_{Q(R,S)}$ for `rand14`. (RHS): $f^S_{Q(S)}$ versus $f^S_{Q(R,S)}$ for `rand14`.

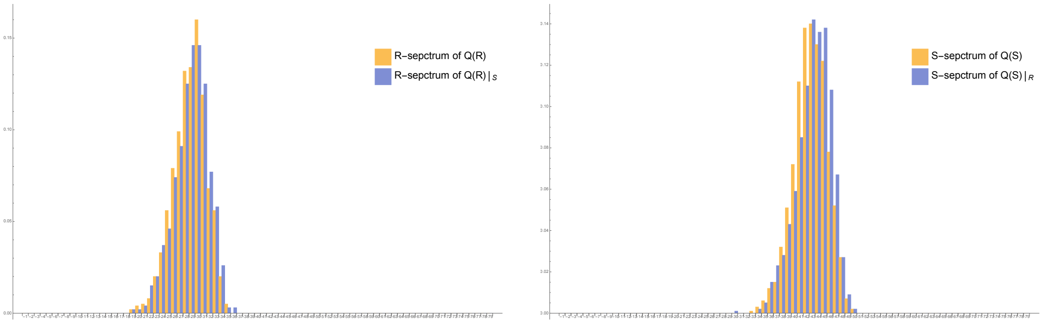


R-spectrum of `rand15` S-spectrum of `rand15`

FIGURE 17. The $R$- and $S$ spectra of the riboswitch structure pair, `rand15`. upper left: $f^R_{Q(R)}$ versus $f^R_{Q(R)|_S}$ for `rand15`. upper right: $f^S_{Q(S)}$ versus $f^S_{Q(S)|_R}$ for `rand15`.

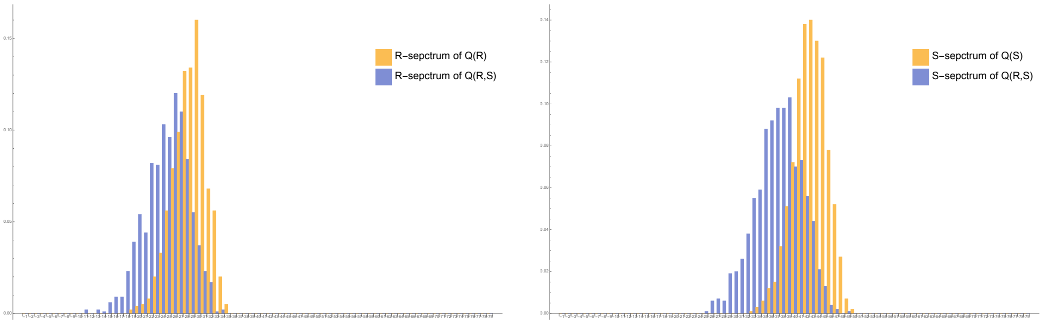


R-spectrum of `rand15` S-spectrum of `rand15`

FIGURE 18. The $R$- and $S$ spectra of the riboswitch structure pair, `rand15`. (LHS): $f^R_{Q(R)}$ versus $f^R_{Q(R,S)}$ for `rand15`. (RHS): $f^S_{Q(S)}$ versus $f^S_{Q(R,S)}$ for `rand15`.
